# Supplementary material for: Differentially Private Timeseries Forecasts for Networked Control
Source: arXiv:2210.00358 source file (2023-03-09)
Supplement: Supplementary file 1 [file Appendix.tex]

\subsection{Experiments Settings}

\input{figure_latex/arima_exp_table}
